# Supplementary material for: Hartree-Fock Critical Nuclear Charge in Two-Electron Atoms
Source: arXiv:2101.02445 source file (2021-01-07)
Supplement: Supplementary file 1 [file SupportingInformation.pdf]

# Hartree–Fock Critical Nuclear Charge in Two-Electron Atoms: Supporting Information

Hugh G. A. Burton*
*Physical and Theoretical Chemical Laboratory, Department of Chemistry, University of Oxford, Oxford, OX1 3QZ, U.K.*
(Dated: January 6, 2021)

## I. LAGUERRE-BASED ONE- AND TWO-ELECTRON INTEGRALS

We follow Ref. 1 and employ a spatial basis comprised of the spherically-symmetric Laguerre-based functions

$$\chi_\mu(\boldsymbol{r}) = \exp\!\left(-\frac{Ar}{2}\right) L_\mu^{(1)}(Ar), \tag{1}$$

where $L_\mu^{(1)}$ denotes an associated Laguerre polynomial of order $\mu$. Using these basis functions allows analytic expressions for the one- and two-electron integrals to be derived for the numerical Hartree–Fock calculations. However, in contrast to Ref. 1, we use the associated Laguerre polynomials as they lead to fewer recurrence relations in the corresponding matrix elements. Here, we derive these analytic expressions for the overlap, kinetic-energy, electron-nuclear attraction, and two-electron repulsion integrals.

### A. Overlap Integrals

First consider the overlap matrix elements

$$S_{\mu\nu} = \langle \chi_\mu | \chi_\nu \rangle = \int_0^{2\pi} \int_0^{\pi} \int_0^{\infty} \mathrm{e}^{-Ar}\, L_\mu^{(1)}(Ar)\, L_\nu^{(1)}(Ar)\, r^2 \sin\theta \,\mathrm{d}r\,\mathrm{d}\theta\,\mathrm{d}\phi. \tag{2}$$

Introducing the scaled distance $\tilde{r} = Ar$ reduces this integral to the form

$$S_{\mu\nu} = \frac{4\pi}{A^3} \int_0^{\infty} \mathrm{e}^{-\tilde{r}}\, L_\mu^{(1)}(\tilde{r})\, L_\nu^{(1)}(\tilde{r})\, \tilde{r}^2\, \mathrm{d}\tilde{r}, \tag{3}$$

The integral over $\tilde{r}$ can be evaluated by exploiting the recurrence relationship

$$\tilde{r} L_\mu^{(1)}(\tilde{r}) = -(\mu+1) L_{\mu+1}^{(1)}(\tilde{r}) + 2(\mu+1) L_\mu^{(1)}(\tilde{r}) - (\mu+1) L_{\mu-1}^{(1)}(\tilde{r}) \tag{4}$$

in combination with the orthogonality condition[2]

$$\int_0^{\infty} \tilde{r}\, \mathrm{e}^{-\tilde{r}}\, L_\mu^{(1)}(\tilde{r})\, L_\nu^{(1)}(\tilde{r})\, \mathrm{d}\tilde{r} = (\mu+1)\delta_{\mu,\nu} \tag{5}$$

to give

$$S_{\mu\nu} = \frac{4\pi}{A^3}(\mu+1)(\nu+1)\Big(-\delta_{\mu,\nu+1} + 2\delta_{\mu,\nu} - \delta_{\mu,\nu-1}\Big). \tag{6}$$

Here, it should be noted that the basis functions do not form an orthonormalised basis.

### B. Kinetic Energy

The kinetic energy matrix elements are given by

$$T_{\mu\nu} = -\frac{1}{2} \int_0^{2\pi} \int_0^{\pi} \int_0^{\infty} \mathrm{e}^{-\frac{Ar}{2}} L_\mu^{(1)}(Ar)\, \boldsymbol{\nabla}^2 \Big[ L_\nu^{(1)}(Ar)\, \mathrm{e}^{-\frac{Ar}{2}} \Big] r^2 \sin\theta \,\mathrm{d}r\,\mathrm{d}\theta\,\mathrm{d}\phi, \tag{7}$$

where $\boldsymbol{\nabla}^2$ is the Laplacian operator. Since the wave function is defined with no angular component, this Laplacian can be expressed in the scaled electron-nuclear distance $\tilde{r}$ as

$$\boldsymbol{\nabla}^2 = A^2 \left( \frac{\partial^2}{\partial \tilde{r}^2} + \frac{2}{\tilde{r}} \frac{\partial}{\partial \tilde{r}} \right). \tag{8}$$

Eq. (7) then reduces to the one-dimensional integral

$$T_{\mu\nu} = -\frac{2\pi}{A}\int_0^\infty \mathrm{e}^{-\tilde{r}} L_\mu^{(1)}(\tilde{r})\left(\frac{\mathrm{d}^2 L_\nu^{(1)}(\tilde{r})}{\mathrm{d}\tilde{r}^2} + \left(\frac{2}{\tilde{r}} - 1\right)\frac{\mathrm{d}L_\nu^{(1)}(\tilde{r})}{\mathrm{d}\tilde{r}} + \left(\frac{1}{4} - \frac{1}{\tilde{r}}\right)L_\nu^{(1)}(\tilde{r})\right)\tilde{r}^2\,\mathrm{d}\tilde{r}. \tag{9}$$

Exploiting the additional recurrence relations

$$\tilde{r}\,\frac{\mathrm{d}L_\mu^{(1)}(\tilde{r})}{\mathrm{d}\tilde{r}} = \mu L_\mu^{(1)}(\tilde{r}) - (\mu+1)L_{\mu-1}^{(1)}(\tilde{r}), \tag{10a}$$

$$\tilde{r}\,\frac{\mathrm{d}^2 L_\mu^{(1)}(\tilde{r})}{\mathrm{d}\tilde{r}^2} = (\tilde{r}-2)\frac{\mathrm{d}L_\mu^{(1)}(\tilde{r})}{\mathrm{d}\tilde{r}} - \mu L_\mu^{(1)}(\tilde{r}), \tag{10b}$$

yields

$$T_{\mu\nu} = -\frac{2\pi}{A}\int_0^\infty \mathrm{e}^{-\tilde{r}} L_\mu^{(1)}(\tilde{r})\left(\frac{\tilde{r}}{4}L_\nu^{(1)}(\tilde{r}) - (\nu+1)L_\nu^{(1)}(\tilde{r})\right)\tilde{r}\,\mathrm{d}\tilde{r}. \tag{11}$$

Orthogonality and the overlap integral [Eq. (6)] then allows the kinetic-energy to be reduced to the tri-diagonal form

$$T_{\mu\nu} = \frac{\pi}{2A}(\mu+1)(\nu+1)\left(\delta_{\mu,\nu+1} + 2\,\delta_{\mu,\nu} + \delta_{\mu,\nu-1}\right). \tag{12}$$

### C. Electron-Nuclear Attraction

The one-electron potential energy contains only the Coulomb interaction to the nucleus and is given by

$$\begin{aligned} h_{\mu\nu} &= -\int_0^{2\pi}\int_0^{\pi}\int_0^\infty \mathrm{e}^{-Ar}\,L_\mu^{(1)}(Ar)\,\frac{Z}{r}\,L_\nu^{(1)}(Ar)\,r^2\sin\theta\,\mathrm{d}r\,\mathrm{d}\theta\,\mathrm{d}\phi \\ &= -4\pi\frac{Z}{A^2}\int_0^\infty \mathrm{e}^{-\tilde{r}}L_\mu^{(1)}(\tilde{r})\,L_\nu^{(1)}(\tilde{r})\,\tilde{r}\,\mathrm{d}\tilde{r}. \end{aligned} \tag{13}$$

This integral matches the orthogonality relation Eq. (5) and thus easily reduces to the diagonal form

$$h_{\mu\nu} = -4\pi\frac{Z}{A^2}(\mu+1)\delta_{\mu\nu}. \tag{14}$$

### D. Two-Electron Integrals

The two-electron repulsion integrals are more challenging to derive, but analytic forms are possible.[1] We loosely follow the derivation outlined in Ref. 1, although we believe that our derivation provides a simpler analytic form. Consider the two-electron repulsion integral defined as

$$\langle\mu\nu\|\sigma\tau\rangle = \iiint \chi_\mu(\boldsymbol{r}_1)\chi_\nu(\boldsymbol{r}_2)\,\frac{1}{|\boldsymbol{r}_1 - \boldsymbol{r}_2|}\,\chi_\sigma(\boldsymbol{r}_1)\chi_\tau(\boldsymbol{r}_2)\,\mathrm{d}\boldsymbol{r}_1\mathrm{d}\boldsymbol{r}_2. \tag{15}$$

Using the Laguerre-based polynomials, this integrals takes the form

$$\langle\mu\nu\|\sigma\tau\rangle = \iiint \mathrm{e}^{-A(r_1+r_2)}L_\mu^{(1)}(Ar_1)\,L_\nu^{(1)}(Ar_2)\,\frac{1}{r_{12}}\,L_\sigma^{(1)}(Ar_1)\,L_\tau^{(1)}(Ar_2)\,\mathrm{d}\boldsymbol{r}_1\mathrm{d}\boldsymbol{r}_2. \tag{16}$$

First, we trasnform to the $A$-scaled perimetric coordinate system[1]

$$z_1 = A(r_2 + r_{12} - r_1), \tag{17a}$$

$$z_2 = A(r_{12} + r_1 - r_2), \tag{17b}$$

$$z_3 = A(r_1 + r_2 - r_{12}), \tag{17c}$$

with the Jacobian

$$\mathrm{d}\boldsymbol{r}_1\mathrm{d}\boldsymbol{r}_2 = \frac{\pi^2}{4A^6}(z_2+z_3)(z_1+z_3)(z_1+z_2)\mathrm{d}z_1\mathrm{d}z_2\mathrm{d}z_3. \tag{18}$$

In this coordinate system, the two-electron integrals reduce to the form

$$\langle \mu\nu \| \sigma\tau \rangle = \frac{\pi^2}{2A^5} \int_0^\infty \int_0^\infty \int_0^\infty \mathrm{e}^{-(z_1+z_2+2z_3)/2} L_\mu^{(1)}\left(\frac{z_2+z_3}{2}\right) L_\nu^{(1)}\left(\frac{z_1+z_3}{2}\right) L_\sigma^{(1)}\left(\frac{z_2+z_3}{2}\right) L_\tau^{(1)}\left(\frac{z_1+z_3}{2}\right) (z_1+z_3)(z_2+z_3)\,\mathrm{d}z_1\mathrm{d}z_2\mathrm{d}z_3. \tag{19}$$

The associated Laguerre polynomials can be expressed explicitly as

$$L_\mu^{(1)}(z) = \sum_{\mu_i=0}^{\mu} \frac{(-1)^{\mu_i}}{\mu_i!} \binom{\mu+1}{\mu-\mu_i} z^{\mu_i}, \tag{20}$$

giving the two-electron integrals as

$$\begin{aligned} \langle \mu\nu \| \sigma\tau \rangle = \frac{\pi^2}{2A^5} \int_0^\infty \int_0^\infty \int_0^\infty & \mathrm{d}z_1\mathrm{d}z_2\mathrm{d}z_3\, \mathrm{e}^{-(z_1+z_2+2z_3)/2} \\ & \times \sum_{\mu_i,\nu_i,\sigma_i,\tau_i=0}^{\mu,\nu,\sigma,\tau} \left(-\frac{1}{2}\right)^{\phi} \frac{1}{\mu_i!\nu_i!\sigma_i!\tau_i!} \binom{\mu+1}{\mu-\mu_i}\binom{\nu+1}{\nu-\nu_i}\binom{\sigma+1}{\sigma-\sigma_i}\binom{\tau+1}{\tau-\tau_i} (z_2+z_3)^{\mu_i+\sigma_i+1}(z_1+z_3)^{\nu_i+\tau_i+1} \end{aligned} \tag{21}$$

where $\phi = \mu_i + \nu_i + \sigma_i + \tau_i$. Expanding the terms $(z_2+z_3)^{\mu_i+\sigma_i+1}$ and $(z_1+z_3)^{\nu_i+\tau_i+1}$ allows the triple integral to be separated as

$$\begin{aligned} \langle \mu\nu \| \sigma\tau \rangle = \frac{\pi^2}{2A^5} \sum_{\mu_i,\nu_i,\sigma_i,\tau_i=0}^{\mu,\nu,\sigma,\tau} \sum_{a=0}^{\nu_i+\tau_i+1} \sum_{b=0}^{\mu_i+\sigma_i+1} & \left(-\frac{1}{2}\right)^{\phi} \frac{1}{\mu_i!\nu_i!\sigma_i!\tau_i!} \binom{\nu_i+\tau_i+1}{a}\binom{\mu_i+\sigma_i+1}{b}\binom{\mu+1}{\mu-\mu_i}\binom{\nu+1}{\nu-\nu_i}\binom{\sigma+1}{\sigma-\sigma_i}\binom{\tau+1}{\tau-\tau_i} \\ & \times \int_0^\infty \mathrm{e}^{-z_1/2} z_1^{1+\nu_i+\tau_i-a}\,\mathrm{d}z_1 \int_0^\infty \mathrm{e}^{-z_2/2} z_2^{1+\mu_i+\sigma_i-b}\,\mathrm{d}z_2 \int_0^\infty \mathrm{e}^{-z_3} z_3^{a+b}\,\mathrm{d}z_3. \end{aligned} \tag{22}$$

Each constituent integral can be evaluated using the Euler integral[2] for positive integers $n$

$$\int_0^\infty t^n\, \mathrm{e}^{-\alpha t}\,\mathrm{d}t = \alpha^{-(n+1)} n! \tag{23}$$

giving the simplified form

$$\begin{aligned} \langle \mu\nu \| \sigma\tau \rangle = \frac{8\pi^2}{A^5} \sum_{\mu_i,\nu_i,\sigma_i,\tau_i=0}^{\mu,\nu,\sigma,\tau} \sum_{a=0}^{\nu_i+\tau_i+1} \sum_{b=0}^{\mu_i+\sigma_i+1} & (-1)^{\phi} \frac{1}{\mu_i!\nu_i!\sigma_i!\tau_i!} \binom{\nu_i+\tau_i+1}{a}\binom{\mu_i+\sigma_i+1}{b}\binom{\mu+1}{\mu-\mu_i}\binom{\nu+1}{\nu-\nu_i}\binom{\sigma+1}{\sigma-\sigma_i}\binom{\tau+1}{\tau-\tau_i} \\ & \times \left(\frac{1}{2}\right)^{(a+b)} (\nu_i+\tau_i+1-a)!\,(\mu_i+\sigma_i+1-b)!\,(a+b)! \end{aligned} \tag{24}$$

All the factorial terms can then be removed by noting that

$$\frac{1}{\mu_i!\nu_i!\sigma_i!\tau_i!} \binom{\nu_i+\tau_i+1}{a}\binom{\mu_i+\sigma_i+1}{b} (\nu_i+\tau_i+1-a)!\,(\mu_i+\sigma_i+1-b)!\,(a+b)! \;=\; (\mu_i+\sigma_i+1)(\nu_i+\tau_i+1)\binom{\mu_i}{\sigma_i}\binom{\nu_i}{\tau_i}\binom{a}{b}. \tag{25}$$

The analytic two-electron integrals are therefore given purely as a weighted summation of products of binomial coefficients

$$\langle \mu\nu \| \sigma\tau \rangle = \frac{8\pi^2}{A^5} \sum_{\mu_i,\nu_i,\sigma_i,\tau_i=0}^{\mu,\nu,\sigma,\tau} \sum_{a=0}^{\nu_i+\tau_i+1} \sum_{b=0}^{\mu_i+\sigma_i+1} (-1)^{\phi} \left(\frac{1}{2}\right)^{(a+b)} (\mu_i+\sigma_i+1)(\nu_i+\tau_i+1) \binom{\nu_i}{\tau_i}\binom{\mu_i}{\sigma_i}\binom{a}{b}\binom{\mu+1}{\mu-\mu_i}\binom{\nu+1}{\nu-\nu_i}\binom{\sigma+1}{\sigma-\sigma_i}\binom{\tau+1}{\tau-\tau_i}. \tag{26}$$

### E. Implementation and Discussion

The analytic integrals presented here can be readily implemented to give highly-accurate matrix elements. Significantly, in each case, we find $A$ and $Z$ only appear as prefactors, and thus once the $\mu, \nu, \sigma, \tau$ dependent terms of the matrix elements have been computed, they can be simply rescaled for different $A$ and $Z$. This scaling offers a major advantage for the two-electron integrals as the computationally expensive nested summations now only need to be explicitly evaluated once. For large basis sets, arbitrary precision is required to handle the binomial coefficients in the two-electron integrals, and thus we make use of the GMP

library.[3] Since all the $\mu, \nu, \sigma, \tau$ dependent components contain only integer or rational terms, these matrix elements are well-suited to this arbitrary precision approach.

* hugh.burton@chem.ox.ac.uk

1 A. W. King, A. L. Baskerville, and H. Cox, Phil. Trans. R. Soc. A **376**, 20170153 (2018).
2 K. F. Riley, M. P. Hobson, and S. J. Bence, *Mathematical Methods for Physics and Engineering* (Cambridge University Press, 2006).
3 T. Granlund and the GMP development team, *GNU MP: The GNU Multiple Precision Arithmetic Library*, 5th ed. (2012), http://gmplib.org.
